# Supplementary material for: New Renormalization Group Results for Scaling of Self-Avoiding Tethered Membranes
Source: arXiv:cond-mat/9608022 source file (1996-07-26)
Supplement: Supplementary file 1 [file appendix.tex]

%auto-ignore
\subsection{Factors from nests}
\label{s:Factors from nests}
\begin{figure}[htb] 
\centerline{ 
    \epsfxsize=14cm \epsfbox{../eps/nest.eps}
}
\caption{The nested subcontractions}
\label{f:wave3}
\end{figure}
We know that combinatorical factors appear for nested contractions.
If a subset of points is contracted towards a marginal operator $O$, it
will appear with a pole in $1/\E$ times the operator $O$. This is only
valid as long as the distances in this subcontraction are smaller than the
distances in the rest of the diagram. This statement is rather vague.
Formally it can be precized in the following way. To calculate the
associated number (the pole terms + finite terms) of the subcontraction
the usual regularization prescription shall be taken, i.e. all 
the distances have to be borned by say $l$. Then the result is 
the usual diagram times $l^\E$. This diagram is imbedded in some
larger diagram, which is calculated by demanding that all the distances
are smaller than $L$. The associated counterterm shall then be the 
factors given by the MOPE times $\Theta(L>l)$. This results in 
exactly a factor $1/2$ in comparison to the simple product
of the two diagrams, which account for the nest.
